# Supplementary material for: Gapped spin-1/2 spinon excitations in a new kagome quantum spin liquid compound Cu$_3$Zn(OH)$_6$FBr
Source: arXiv:1702.01658 source file (2017-06-23)
Supplement: Supplementary file 1 [file supplementalMaterial.pdf]

# Supplemental Material for "Gapped spin-1/2 spinon excitations in a new kagome quantum spin liquid compound $Cu_3Zn(OH)_6FBr$"

## 1. Fitting of the Knight shift data

Here we discuss the fitting of the Knight shift data using different functions.

In Fig. S1, we employ a function form, $K_{chem}$ + $A$ exp$(-\Delta/T)$, to fit the low temperature data and extract the size of the gap at different fields. The $K_{chem}$ = 0.015% was obtained from the $K$-$\chi$ plot in the inset of Fig. 3(b) of the main text, and $A$ is a free fitting parameter.

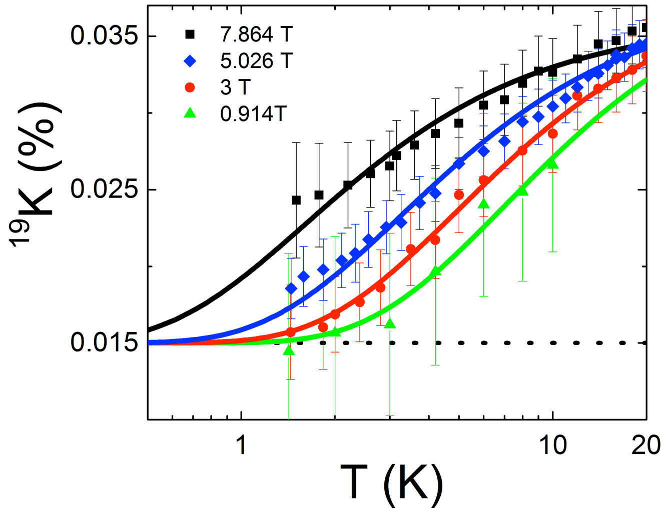


Fig. S1. Knight shift data fitted with $K_{chem}$+$A$ exp($-\Delta/T$).

In the main text, we do not include temperature prefactor in the fitting as in Ref. 29, $K_{chem}$ + $AT$ exp($-\Delta/T$). The reason is following: Knight shift measures the density of states (DOS) which counts the number of low energy levels of excitations. Actually, antiferromagnetic correlations only affect the spectrum weight of the energy levels, but not the number of them. In others words, correlations will change the wave packet of quasi-particles, but do not annihilate or create them.

A trial of fitting our data with, $K_{chem}$ + $AT$ exp($-\Delta/T$), shows that it cannot render a good fit. As shown in Fig. S2, the dashed lines cannot even go through the data points. Moreover, the obtained gap size becomes negative at large fields (can be seen in Tab. S1.), which is irrational. We hence argue, that if one wants to take antiferromagnetic correlations into account, a Currie-Weiss factor, $C/(T+\theta)$, should be used, namely, $K_{chem}$+$C/(T+\theta)$exp($-\Delta/T$). The corresponding results are shown in Fig. S3 in which data points over a much wider temperature range fit to the function. The gap size obtained by using different fitting functions are summarized in the Tab. S1. The $\Delta$ obtained from a fitting to $K_{chem}$+$C/(T+\theta)$exp($-\Delta/T$) is slightly larger than that obtained from the fitting to $K_{chem}$ +A*exp($-\Delta$/T), but the magnetic field dependence of the gap size is the same, as can be in Fig. S4. To be more conservative on the estimate of the gap size, in the main text we use the fitting form,

$K_{chem}+A\ \exp(-\Delta/T)$, which gives a smaller $\Delta$.

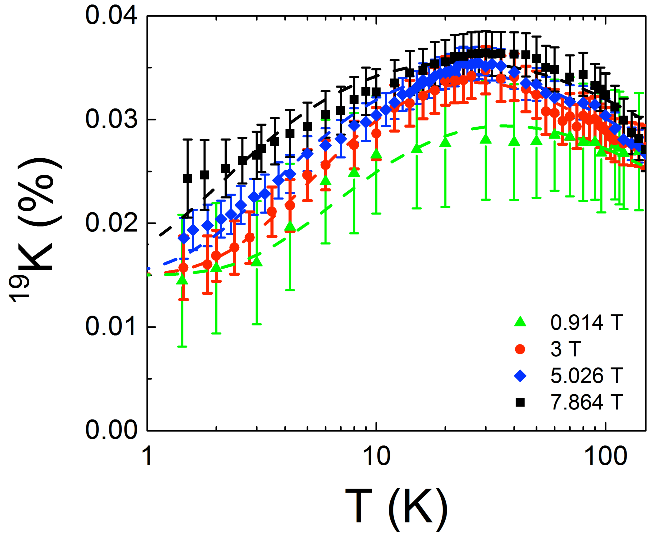


Fig. S2. Knight shift data fitted with $K_{chem} + AT\ \exp(-\Delta/T)$.

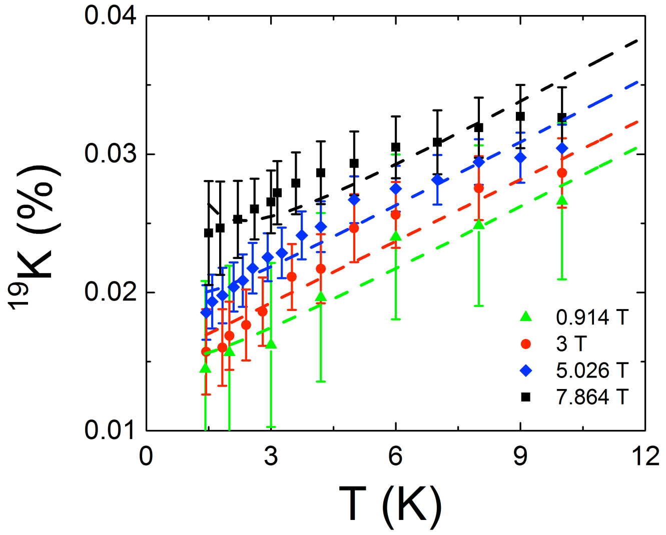


Fig. S3. Knight shift data fitted with $K_{chem}+C/(T+\theta)\exp(-\Delta/T)$.

| $H$ (T) | $\Delta$ obtained from different fitting functions | |
|---|---|---|
| | $K_{chem} + AT\ \exp(-\Delta/T)$ | $K_{chem}+C/(T+\theta)\exp(-\Delta/T)$ |
| 0.914 | 1.90±1.43 | 7.18±0.41 |
| 3 | 0.15±0.53 | 5.65±0.23 |
| 5.026 | -1.17±0.21 | 3.81±0.16 |
| 7.864 | -2.32±0.20 | 2.16±0.16 |

Tab. S1. The gap value obtained from two different fitting schemes.

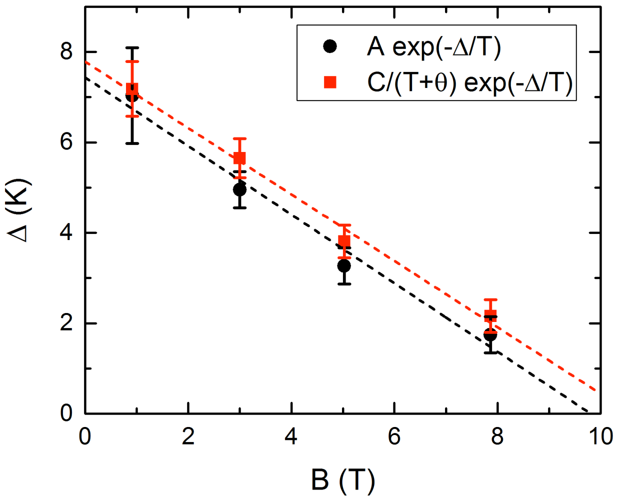


Fig. S4. Gap size obtained from two different fitting forms are consistent with each other.

## 2. Knight shift and magnetic susceptibility as a function of temperature

In Fig. S5, we compare the temperature dependence of macroscopic susceptibility data (red squares) and the Knight shift data (black circles) at magnetic field $B$=3 T. It is clearly seen that they scale one another at high temperatures of $T$>75 K.

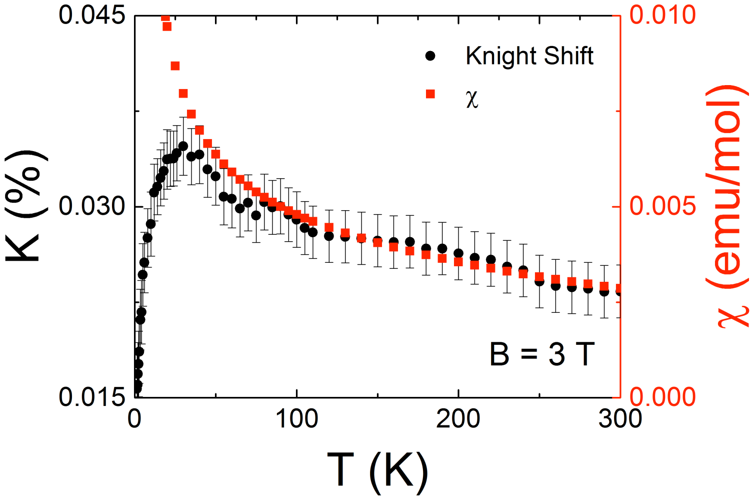


Fig. S5. Comparison of macroscopic susceptibility and the Knight shift data.

## 3. No contribution from free spins evidenced by spectra with different $\tau$

In the Fig. 3 (a) of the main text, the spectra become slightly asymmetric and a bit wider at 55 K. To explore the possible reason behind this, we have performed further NMR measurements with different pulse interval ($\tau$) at $T$=55 K and 4.2 K. The results are shown in Fig. S5 (a) and (b). The spectra become asymmetric at 55 K and this fact is attributed to magnetic anisotropy as mentioned in the main text. To confirm that the shoulder is not from free spins due to defect which should have a shorter spin-spin relaxation time $T_2$, we compare the lineshape measured with

different $\tau$. If there is contribution due to free spins due to defect or other magnetic impurities, the spectra will become sharper with longer $\tau$, as in the work by M. Fu, T. Imai, T.-H. Han, Y.S. Lee, (Science 350 (2015) 655.) Fig. S4. However, our spectra do not become sharper when using longer $\tau$, which proves that our spectra have no such contribution. The small increase of the shoulder with longer $\tau$ can be understood as due to an anisotropy of $T_2$.

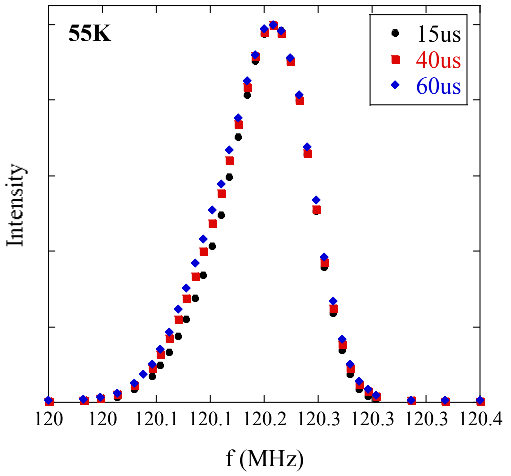


Fig. S6. (a) Spectra measured with different $\tau$ at 55K.

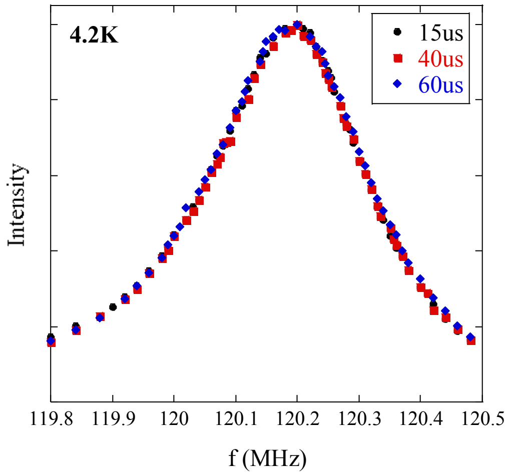


Fig. S6. (b) Spectra measured with different $\tau$ at 4.2K.

## 4. AC susceptibility at different frequencies

One may worry that the broadening of the NMR spectra at low temperatures could be caused by a formation of spin glass. To exclude the possibility of glassy behavior in our material, we have further performed magnetic susceptibility measurements at different frequencies. As shown in Fig. S7, at $B$=1 T and $B$=5 T, the temperature dependence of the magnetic susceptibility shows no frequency dependence, which safely rules out the possibility of spin glass behavior in our material.

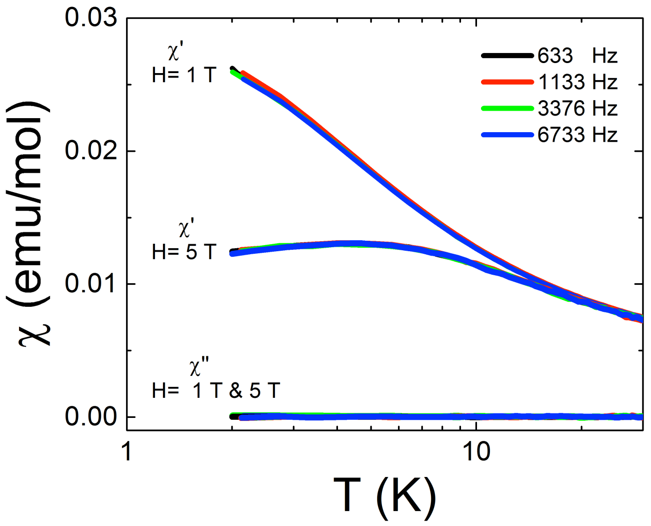


Fig. S7. Temperature dependence of the magnetic susceptibility at different magnetic fields and different frequencies. Clearly, no sign of spin glass type of slow dynamics can be seen.

Moreover, in Fig. S7, besides the real part of magnetic susceptibility $\chi$', we have also shown the imaginary part $\chi$'', and it is zero throughout, which also means there is no dissipation of our system due to spin glass or other mechanism.
